# Supplementary material for: The Fourth S-PLUS Data Release: 12-filter photometry covering $\sim3000$ square degrees in the southern hemisphere
Source: arXiv:2407.20701 source file (2024-07-30)
Supplement: Supplementary file 1 [file appendix-institutions.tex]

\section{Authors affiliations}\label{ap:affiliations}

$^{1}$ Cambridge Survey Astronomical Unit (CASU), Insitute of Astronomy, University of Cambridge, Madingley Road, Cambridge, CB3 0HA, GB

\noindent
$^{2}$ Instituto de Astronomia, Geofísica e Ciências Atmosféricas, Rua do Matão, 1226, Cidade Universitária, São Paulo, 05508-090, BR

\noindent
$^{3}$ Universidade Presbiteriana Mackenzie, Rua da Consolação, 930, Consolação, São Paulo, 01302-907, BR

\noindent
$^{4}$ University of Washington, 1415 NE 45th St, Seattle, 98195, US

\noindent
$^{5}$ Centro de Astronomía (CITEVA), Universidad de Antofagasta, Av. Angamos 601, Antofagasta, 1240000, CL

\noindent
$^{6}$ Millennium Institute of Astrophysics, Nuncio Monse\~nor Sotero Sanz 100, Of. 104, Providencia, 750-0000, CL

\noindent
$^{7}$ Laboratório Nacional de Astrofísica, Rua Estados Unidos, 154, Itajubá, 37504-364, BR

\noindent
$^{8}$ Instituto de Astrofísica de Canarias, C/ Vía Láctea s/n, La Laguna, 38205, ES

\noindent
$^{9}$ Universidade Federal de Santa Catarina, Campus Universitário Reitor João David Ferreira Lima, Florianópolis, 88040-900, BR

\noindent
$^{10}$ Giant Magellan Telescope, 251 S. Lake Ave, Suite 300, Pasadena, 91101, US

\noindent
$^{11}$ INAF - Osservatorio Astronomico di Padova, Vicolo dell'Osservatorio, 5, Padova, 35122, IT

\noindent
$^{12}$ Observatório Nacional, Rua General José Cristino, 77, Bairro São Cristóvão, Rio de Janeiro, 20921-400, BR

\noindent
$^{13}$ Instituto de Astrofísica de La Plata, UNLP-CONICET, Paseo del Bosque s/n, La Plata, B1900FWA, AR

\noindent
$^{14}$ Facultad de Ciencias Astronómicas y Geofísicas, Universidad Nacional de La Plata, Paseo del Bosque s/n, La Plata, B1900FWA, AR

\noindent
$^{15}$ Centro Universitário FEI, Av. Humberto de Alencar Castelo Branco, 3972, São Bernardo do Campo, 09850-901, BR

\noindent
$^{16}$ Nicolaus Copernicus Astronomical Center, Polish Academy of Sciences, Bartycka 18, Warsaw, 00-716, PL

\noindent
$^{17}$ Instituto de Astronomía y Ciencias Planetarias, Universidad de Atacama, Copayapu 485, Copiapó, 1530000, CL

\noindent
$^{18}$ Centro Brasileiro de Pesquisas Físicas, Rua Dr. Xavier Sigaud, 150, Rio de Janeiro, 22290-180, BR

\noindent
$^{19}$ Centro Federal de Educação Tecnológica Celso Suckow da Fonseca, Rodovia Mário Covas, lote J2, quadra J, Itaguaí, 23810-000, BR

\noindent
$^{20}$ Universidade Federal do Rio Grande do Sul, Av. Bento Gonçalves, 9500, Porto Alegre, 91501-970, BR

\noindent
$^{21}$ Observatório do Valongo, Ladeira Pedro Antônio, 43, Saúde, Rio de Janeiro, 20080-090, BR

\noindent
$^{22}$ Departamento de Astronomía, Universidad de La Serena, Raúl Bitrán 1305, La Serena, , CL

\noindent
$^{23}$ Instituto de Matemática e Estatística, Rua do Matão, 1010, Cidade Universitária, São Paulo, 05508-090, BR

\noindent
$^{24}$ Instituto Multidisciplinario de Investigación y Postgrado, Universidad de La Serena, Raúl Bitrán 1305, La Serena, 1720236, CL

\noindent
$^{25}$ Departamento de Física, Universidade Federal de Sergipe, Av. Marechal Rondon, s/n, São Cristóvão, 49100-000, BR

\noindent
$^{26}$ Southern Astrophysical Research Telescope, Cerro Pachón, La Serena, 1720236, CL

\noindent
$^{27}$ Leiden Observatory, University of Leiden, Niels Bohrweg 2, Leiden, 2333 CA, NL

\noindent
$^{28}$ TNO, Oude Waalsdorperweg 63, Den Haag, 2597 AK, NL

\noindent
$^{29}$ NFS's NOIRLab, 950 N. Cherry Ave, Tucson, 85719, US

\noindent
$^{30}$ Department of Physics and Astronomy and JINA Center for the Evolution of the Elements (JINA-CEE), 225 Nieuwland Science Hall, Notre Dame, 46556, US

\noindent
$^{31}$ Institute for Astronomy, Astrophysics, Space Applications and Remote Sensing, National Observatory of Athens, I. Metaxa \& Vas. Pavlou, Palaia Penteli, 15236, GR

\noindent
$^{32}$ Department of Astronomy \& Steward Observatory, University of Arizona, 933 N. Cherry Ave, Tucson, 85721, US

\noindent
$^{33}$ Rubin Observatory Project Office, 950 N. Cherry Ave, Tucson, 85719, US
